# Supplementary material for: Reactive Informative Planning for Mobile Manipulation Tasks under Sensing and Environmental Uncertainty
Source: arXiv:2205.06301 source file (2022-05-12)
Supplement: Supplementary file 1 [file appendix_LTL.tex]

%  symbolic controller
%\pagebreak
\section{Detailed Description of the Symbolic Controller}
\label{appendix:ltl_planner}
%\robotpositionunicycle(0),\workspace(0)
%%
%
This Appendix provides a detailed description of the distance metric used in Section~\ref{sec:ltl_planner} upon which a discrete controller is designed that generates manipulation commands online. To accomplish this, first in Appendix~\ref{sec:nbaAp} we translate the LTL formula into a Non-deterministic B$\ddot{\text{u}}$chi Automaton (NBA) and we provide a formal definition of its accepting condition. 
Then, in Appendix~\ref{sec:dist}, we provide a detailed description for the construction of the distance metric over this automaton state space. Appendix~\ref{appendix:planning} describes our method for generating symbolic actions online, and Appendix~\ref{appendix:completeness} includes the proof of our completeness result. The proposed method is also illustrated in Figs.~\ref{fig:NBA}-\ref{fig:graphG}.
%We also provide conditions under which the discrete controller is complete, in the sense that if there exists a feasible solution, then if the continuous-time controller can always execute the manipulation commands generated by the discrete controller, then the LTL task will be satisfied. 

%(e.g., `go to region $\ell_j$ and grasp object $\movableobjectdilated_i$'). %The detailed construction of this metric is along the lines of the algorithm proposed in [cite ICRA]\footnote{there are some differences because we have atomic propositions based on robot actions; so this needs to be discussed in the final version. Also, here we have a single robot which simplifies the ICRA algorithm}.
%we convert this automaton into a graph structure that captures the NBA transitions that can be enabled if local reachability problems are solved. The conversion process is presented in Appendix A.  Finally

\subsection{From LTL Formulas to Automata}\label{sec:nbaAp}

\begin{figure}[t]
  \centering
  \captionsetup{width=\linewidth,font=footnotesize}
  \includegraphics[width=0.6\linewidth]{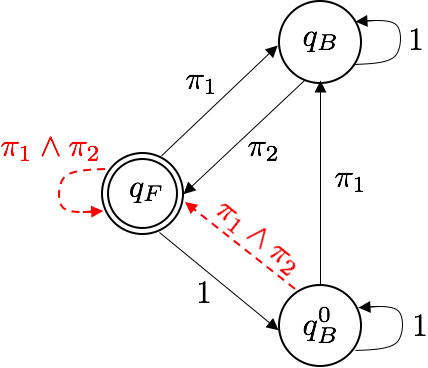}
  \caption{Graphical illustration of the NBA corresponding to the LTL formula $\phi=\square\Diamond(\pi_1)\wedge\square\Diamond(\pi_2)$ where for simplicity of notation $\pi_1=\pi^{a_1(\varnothing, \ell_1)}$ and $\pi_2=\pi^{a_1(\varnothing, \ell_2)}$. The automaton has been generated using the tool in \cite{gastin2001fast}. In words, this LTL formula requires the robot to visit infinitely often and in any order the regions $\ell_1$ and $\ell_2$. The initial state of the automaton is denoted by $q_B^0$ while the final state is denoted by $q_F$. When the robot is in an NBA state and the Boolean formula associated with an outgoing transition from this NBA state is satisfied, then this transition can be enabled. For instance, when the robot is in the initial state $q_B^0$ and satisfies the atomic predicate $\pi_1$, the transition from $q_B^0$ to $q_B$ can be enabled, i.e., $q_B\in\delta_B(q_B^0,\pi_1)$. The LTL formula is satisfied if starting from $q_B^0$, the robot generates an infinite sequence of observations (i.e., atomic predicates that become true) that yields an infinite sequence of transitions so that the final state $q_F$ is visited infinitely often. The red dashed lines correspond to infeasible NBA transitions as they are enabled only if the Boolean formula $\pi_1\wedge\pi_2$ is satisfied, i.e., only if the robot is in more than one region simultaneously; such edges are removed yielding the pruned NBA. }
  \label{fig:NBA}
\end{figure}

As reported in Section~\ref{sec:ltl_planner}, we first translate the specification $\phi$, constructed using a set of atomic predicates $\mathcal{AP}$, into a Non-deterministic B$\ddot{\text{u}}$chi Automaton (NBA) defined as follows; see also Fig.~\ref{fig:NBA}. %Given a temporal logic formula $\phi$ , with syntax and semantics as described in Definitions~\ref{syntax} and \ref{semantics}, respectively, a DFA is defined as follows:
 \begin{definition}[NBA]
 A Non-deterministic B$\ddot{\text{u}}$chi Automaton (NBA) $B$ over $\Sigma=2^{\mathcal{AP}}$ is defined as a tuple $B=\left(\ccalQ_{B}, \ccalQ_{B}^0,\delta_B, \ccalQ_F\right)$, where (i) $\ccalQ_{B}$ is the set of states;
 (ii) $\ccalQ_{B}^0\subseteq\ccalQ_{B}$ is a set of initial states; (iii) $\delta_B:\ccalQ_B\times\Sigma\rightarrow 2^{\ccalQ_B}$ is a non-deterministic transition relation, and $\ccalQ_F\subseteq\ccalQ_{B}$ is a set of accepting/final states.
 \label{def:nba}
 \end{definition}
To interpret a temporal logic formula over the trajectories of the robot system, we use a labeling function $L:\ccalA\rightarrow 2^{\mathcal{AP}}$ that determines which atomic propositions are true given the current robot action $a_k(\movableobjectdilated_i,\ell_j)$; note that, by definition, these actions also encapsulate the position of the robot in the environment.
%%
%
%An infinite-length discrete plan $\tau=\tau(0)\tau(1)\dots$ satisfies $\phi$, denoted by $\tau\models\phi$, if the word $\sigma=L(\tau(0))L(\tau(1))\dots$ yields an accepting NBA run defined as follows. First, a run of $\rho_B$ of $B$ over an infinite word $\sigma=\sigma(1)\sigma(2)\dots\sigma(t)\dots\in(2^{\mathcal{AP}})^{\omega}$, is a sequence $\rho_B=q_B(0)q_B(1)q_B(2)\dots,q_B(t),\dots$, where $q_B(0)\in\ccalQ_B^0$ and $\delta_B(q_B(t),\sigma(t),q_B(t+1)$, $\forall t\in\mathbb{N}$. %Hereafter, we equivalently denote $\delta_B(q_B(t),\sigma(t),q_B(t+1)$ as $q_B(t)\rightarrow_B q_B(t+1)$. A run $\rho_B$ is called \textit{accepting} if at least one final state appears infinitely often in it. In words, an infinite-length discrete plan $\tau$ satisfies an LTL formula $\phi$ if it can generate at least one accepting NBA run. Hereafter, for simplicity we replace $L(\bbp(t),M(t))$ with $L(\bbp(t))$.
%
%
An infinite sequence $p=p(0)p(1)\dots p(k)\dots$ of actions $p(k)\in\ccalA$, satisfies $\phi$ if the word $\sigma=L(p(0))L(p(1))\dots$ yields an accepting NBA run defined as follows \cite{baier2008principles}. First, a run $\rho_B$ of $B$ over an infinite word $\sigma=\sigma(1)\sigma(2)\dots\sigma(k)\dots\in(2^{\mathcal{AP}})^{\omega}$, is a sequence $\rho_B=q_B^0q_B^1q_B^2\dots,q_B^k,\dots$, where $q_B^0\in\ccalQ_B^0$ and $q_B^{k+1}\in\delta_B(q_B^k,\sigma(k))$, $\forall k\in\mathbb{N}$. A run $\rho_B$ is called \textit{accepting} if at least one final state appears infinitely often in it. In words, an infinite-length discrete plan $\tau$ satisfies an LTL formula $\phi$ if it can generate at least one accepting NBA run.
%Particularly, if the sequence of observations/symbols generated along $\tau$ defined as $\sigma=L(\tau(0)),L(\tau(1))\dots$ can generate at least one infinite sequence of NBA states, starting from the initial NBA state, that includes at least one of the final states infinitely often, then we say that $\tau$ satisfies $\phi$. %Hereafter, for simplicity we replace $L(\robotpositionunicycle(t),\workspace(t))$ with $L(\robotpositionunicycle(t))$. 

\subsection{Distance Metric Over the NBA}\label{sec:dist}
%\textcolor{red}{[some text/definitions may be removed from the final draft]}

\begin{figure}[t]
  \centering
  \captionsetup{width=\linewidth,font=footnotesize}
  \includegraphics[width=1\linewidth]{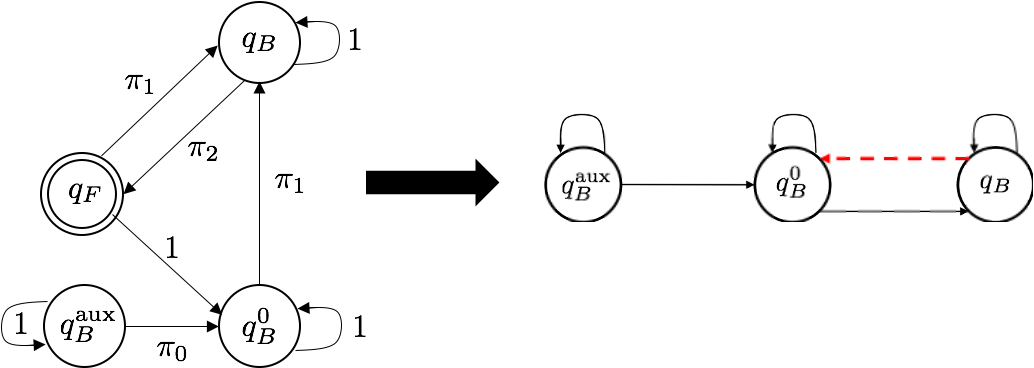}
  \caption{Graphical illustration of the graph $\ccalG$ construction for the NBA shown in Fig.~\ref{fig:NBA}. The left figure corresponds to the pruned automaton after augmenting its state space with the state $q_B^{\text{aux}}$, where $\pi_0$ corresponds to the atomic predicate that the robot satisfies initially at $t=0$. If no atomic predicates are satisfied initially, then $\pi_0$ corresponds to the empty symbol \cite{baier2008principles}. Observe in the left figure that $\ccalD_{q_B^{\text{aux}}}=\{q_B^{\text{aux}},q_B^0,q_B\}$. The right figure illustrates  the graph $\ccalG$ corresponding to this automaton. The red dashed line corresponds to an accepting edge. Also, we have that $\ccalV_F=\{q_B\}$, $d_F(q_B^{\text{aux}},\ccalV_F)=2$, $d_F(q_B^{0},\ccalV_F)=1$, and $d_F(q_B,\ccalV_F)=0$. For instance, every time the robot reaches the state $q_B^0$ with $d_F(q_B^{0},\ccalV_F)=1$, it generates a symbol to reach the state $q_B$ since reaching this state decreases the distance to the set of accepting edges (since $d_F(q_B,\ccalV_F)=0$). The symbol that can enable this transition is the symbol that satisfies the Boolean formula $b^{q_B^0,q_B}=\pi_1$; this formula is trivially satisfied by the symbol $\pi_1=\pi^{a_1(\varnothing, \ell_1)}$. As a result the command send to the continuous time controller is `Move to Region $\ell_1$'. %Also, there are two runs in the form \eqref{eq:run} originating from $q_B$: $\rho_1=q_Bq_B$ and $\rho_2=q_B q_F q_B^0$. Note that the run $\rho=q_B q_F q_B$ cannot be generated as there is no feasible symbol that satisfies $\pi_1^{\ell_1}\wedge\pi_1^{\ell_2}$. In fact, this run requires robot $1$ to `jump' from $\ell_1$ to $\ell_2$ instantaneously.
  }
  \label{fig:graphG}
\end{figure}

In this Section, given a graph constructed using the NBA, we define a function to compute how far an NBA state is from the set of final states.
Following a similar analysis as in \cite{kantaros2018text,kantaros2020reactive}, we first prune the NBA by removing infeasible transitions that can never be enabled as they require the robot to be in more than one region and/or take more that one action simultaneously.  %(ii) we define a distance metric over the pruned automaton that measures how far the robots are from fulfilling the assigned mission. %among all feasible transitions we identify which transitions are decomposable, i.e., they can be enabled if the robot solves reachability-avoidance planning problems. 
Specifically, a symbol $\sigma\in\Sigma:=2^{\mathcal{AP}}$ is \textit{feasible} if and only if $\sigma\not\models b^{\text{inf}}$, where $b^{\text{inf}}$ is a Boolean formula defined as 
%\pi^{a_k(\movableobjectdilated_i,\movableobjectgoal)}
\begin{align}\label{bInfTSi}
b^{\text{inf}}=&[(\vee_{\forall k,r,j,e\neq j}(\pi^{a_k(\cdot,\ell_e)}\wedge\pi^{a_r(\cdot,\ell_j)}))]\nonumber\\
&\bigvee [(\vee_{\forall j, k,r\neq k}(\pi^{a_k(\cdot,\ell_j)}\wedge\pi^{a_r(\cdot,\ell_j)}))]
%b_j^{\text{inf}}=\vee_{\forall r_i}( \vee_{\forall r_e \text{s.t.} r_i \cap r_e=\emptyset} (\pi_j^{r_i}\wedge\pi_j^{r_e})),
\end{align}
In words, $b^{\text{inf}}$ requires the robot to be either present simultaneously in more than one region \textit{or} take more than one action in a given region at the same time. Specifically, the first line requires the robot to be present in locations $\ell_j$ and $\ell_e$, $e\neq j$ and apply the actions $a_k,a_r\in\ccalA$ while the second line requires the robot to take two distinct actions $a_k(\cdot,\ell_j)$ and $a_r(\cdot,\ell_j)$ at the same region $\ell_j$, simultaneously.

Next, we define the sets that collect all feasible symbols that enable a transition from an NBA state $q_B$ to another, not necessarily different, NBA state $q_B'$. This definition relies on the fact that transition from a state $q_B$ to a state $q_B'$ is enabled if a Boolean formula, denoted by $b^{q_B,q_B'}$ and defined over the set of atomic predicates $\mathcal{AP}$, is satisfied. In other words, $q_B'\in\delta_B(q_B,\sigma)$, i.e., $q_B'$ can be reached from the NBA state $q_B$ under the symbol $\sigma$, if $\sigma$  satisfies $b^{q_B,q_B'}$. An NBA transition from $q_B$ to $q_B'$ is infeasible if there are no feasible symbols that satisfy $b^{q_B,q_B'}$. All infeasible NBA transitions are removed yielding a pruned NBA automaton. All feasible symbols that satisfy $b^{q_B,q_B'}$ are collected in the set $\Sigma^{q_B,q_B'}$.

%\subsection{remaining text...}
%In this Section, given a graph constructed using the pruned automaton, we define a function to compute how far an NBA state is from the set of final states. %so that final states are visited infinitely, i.e., the accepting condition of the NBA is satsified.
%This metric will be used in Section~\ref{appendix:planning} to guide planning towards NBA states that are closer to the final states so that final states are visited infinitely, i.e., the accepting condition of the NBA is satisfied.
%By construction of the pruned automaton, for every a state $q_B\in\ccalQ_B^{\text{dec}}$ there exists a symbol that if repeated a finite number of times then another state $q_B'\in\ccalQ_B^{\text{dec}}$ can be visited while this symbol allows to remain in $q_B'$. Also, as discussed before, transition from $q_B$ to $q_B'$ will occur while possibly going through intermediate states but self-loops are
%To this end, we first construct a directed graph $\ccalG=\{\ccalV,\ccalE\}$ as follows. First, to take into account the initial robot state in this process, 
To take into account the initial robot state in the construction of the distance metric, in the pruned automaton we introduce an auxiliary state $q_B^{\text{aux}}$ and transitions from $q_B^{\text{aux}}$ to all initial states $q_B^0\in\ccalQ_B^0$ so that $b^{q_B^{\text{aux}},q_B^{\text{aux}}}=1$ and $b^{q_B^{\text{aux}},q_B^{0}}=\pi_0$, i.e., transition from $q_B^\text{aux}$ to $q_B^0$ can always be enabled based on the atomic predicate that is initially satisfied denoted by $\pi_0$; note that if no predicates are satisfied initially, then $\pi_0$ corresponds to the empty symbol \cite{baier2008principles}. Hereafter, the auxiliary state $q_B^{\text{aux}}$ is considered to be the initial state of the resulting NBA; see also Fig.~\ref{fig:graphG}. %This allows us to exclude NBA transitions that can never be enabled due to the initial robot configuration; see e.g., Figure ??.  

Next, we collect all NBA states that can be reached from $q_B^{\text{aux}}$ in a possibly multi-hop fashion, using a finite sequence of feasible symbols, so that once these states are reached, the robot can always remain in them as long as needed using the same symbol that allowed it to reach this state. Formally, let $\ccalD_{q_B^{\text{aux}}}$ be a set that collects all NBA states $q_B$ (i) that have a feasible self-loop, i.e., $\Sigma^{q_B,q_B}\neq\emptyset$ and (ii) for which there exists a finite and feasible word $w$, i.e., a finite sequence of feasible symbols, so that starting from $q_B^{\text{aux}}$ a finite NBA run $\rho_w$ (i.e., a finite sequence of NBA states) is incurred that ends in $q_B$ and activates the self-loop of $q_B$. In math, $\ccalD_{q_B^{\text{aux}}}$ is defined as:
%$\ccalD_{q_B^{\text{aux}}}$ is defined as:
\begin{align}\label{eq:reach}
    \ccalD_{q_B^{\text{aux}}}=&\{q_B\in\ccalQ_B|\\&(\Sigma^{q_B,q_B}\neq\emptyset)\wedge(\exists w~\text{s.t.}~\rho_{w}=q_B^{\text{aux}}\dots \bar{q}_B q_Bq_B)\nonumber\}.
\end{align}
By definition of $q_B^{\text{aux}}$, we have that $q_B^{\text{aux}}\in\ccalD_{q_B^{\text{aux}}}$.

Among all possible pairs of states in $\ccalD_{q_B^{\text{aux}}}$, we examine which transitions, possibly multi-hop, can be enabled using feasible symbols, so that, once these states are reached, the robot can always remain in them forever using the same symbol that allowed it to reach this state. Formally, consider any two states $q_B, q_B'\in\ccalD_{q_B^{\text{aux}}}$ (i) that are connected through a - possibly multi-hop - path in the NBA, and (ii) for which there exists a symbol, denoted by $\sigma^{q_B,q_B'}$, so that if it is repeated a finite number of times starting from $q_B$, the following finite run can be generated: 
\begin{equation}\label{eq:run}
    \rho=q_B q_B^1\dots q_B^{K-1}q_B^{K}q_B^{K},
\end{equation}
where $q_B'=q_B^K$, for some finite $K>0$. In \eqref{eq:run}, the run is defined so that (i) $q_B^k\neq q_B^{k+1}$, for all $k\in\{1,K-1\}$; (ii) $q_B^{k}\in\delta_B(q_B^k,\sigma^{q_B,q_B'})$ is not valid for all $\forall k\in\{1,\dots,K-1\}$, i.e., the robot cannot remain in any of the intermediate states (if any) that connect $q_B$ to $q_B'$ either because a feasible self-loop does not exist or because $\sigma^{q_B,q_B'}$ cannot activate this self-loop; and (iii) $q_B'\in\delta_B(q_B',\sigma^{q_B,q_B'})$ i.e., there is a feasible loop associated with $q_B'$ that is activated by $\sigma^{q_B,q_B'}$. Due to (iii), the robot can remain in $q_B'$ as long as $\sigma^{q_B,q_B'}$ is generated. The fact that the finite repetition of a \textit{single} symbol needs to generate the run \eqref{eq:run} precludes multi-hop transitions from $q_B$ to $q_B'$ that require the robot to jump from one region of interest to another one instantaneously as such transitions are not meaningful as discussed in Section~\ref{sec:problem_formulation}; see also Fig.~\ref{fig:graphG}. Hereafter, we denote the - potentially multi-hop - transition incurred due to the run \eqref{eq:run} by  $q_B'\in\delta_{B}^m(q_B,\cdot)$.

%Hereafter, we denote by $\delta_B^K(q_B,\cdot,q_B^K)$ the multi-hop NBA transition corresponding to the run \eqref{eq:run}. 
%
Then, we construct the directed graph $\ccalG=\{\ccalV,\ccalE\}$ where $\ccalV\subseteq\ccalQ_B$ is the set of nodes and $\ccalE\subseteq\ccalV\times\ccalV$ is the set of edges. The set of nodes is defined so that $\ccalV=\ccalD_{q_B^{\text{aux}}}$ and the set of edges is defined so that $(q_B,q_B')\in\ccalE$ if there exists a feasible symbol that incurs the run $\rho_w$ defined in \eqref{eq:run}; see also Fig.~\ref{fig:graphG}. 

Given the graph $\ccalG$, we define the following distance metric.

\begin{definition}[Distance Metric]
Let $\ccalG=\{\ccalV,\ccalE\}$ be the directed graph that corresponds to NBA $B$. Then, we define the distance function $d: \ccalV \times \ccalV \rightarrow \mathbb{N}$ as follows
\begin{equation}\label{eq:dist}
d(q_B,q_B')=\left\{
                \begin{array}{ll}
                  |SP_{q_B,q_B'}|, \mbox{if $SP_{q_B,q_B'}$ exists,}\\
                  \infty, ~~~~~~~~~\mbox{otherwise},
                \end{array}
              \right.
\end{equation}
where $SP_{q_B,q_B'}$ denotes the shortest path (in terms of hops) in $\ccalG$ from $q_B$ to $q_B'$ and $|SP_{q_B,q_B'}|$ stands for its cost (number of hops). 
\end{definition}

In words, $d:\ccalV\times\ccalV\rightarrow \mathbb{N}$ returns the minimum number of edges in the graph $\ccalG$ that are required to reach a state $q_B'\in\ccalV$ starting from a state $q_B\in\ccalV$. This metric can be computed using available shortest path algorithms, such the Dijkstra method with worst-case complexity $O(|\ccalE| + |\ccalV|\log|\ccalV|)$. %This function will be used to guide the robots towards locations in the workspace so that eventually a final DFA state is visited, i.e., the LTL formula is satisfied.
%

%\normalsize
%\footnote{In Section~\ref{sec:complOpt}, we provide conditions under which if $d(q_D^0,q_F)=\infty$ then the assigned co-safe LTL task is infeasible}. %; see Sections~\ref{sec:targetDFA}-\ref{sec:paths}.
%
Next, we define the final/accepting edges in $\ccalG$ as follows.
\begin{definition}[Final/Accepting Edges]\label{def:accEdges}
An edge $(q_B,q_B')\in\ccalE$ is called final or accepting if the corresponding multi-hop NBA transition $q_B'\in\delta_B^m(q_B,\cdot)$ includes at least one final state $q_F\in\ccalQ_F$.
\end{definition}

Based on the definition of accepting edges, we define the set $\ccalV_F\subseteq \ccalV$ that collects all states $q_B\in\ccalV$ from which an accepting edge originates, i.e.,
\begin{equation}\label{eq:accNode}
    \ccalV_F = \{q_B\in\ccalV~|~\exists~ \text{accepting edge}~(q_B,q_B')\in\ccalE \}.
\end{equation}
By definition of the accepting condition of the NBA, we have that if at least one of the accepting edges is traversed infinitely often, then the corresponding LTL formula is satisfied. %States $q_B\in\ccalQ_B^{\text{dec}}$ for which there are accepting edges $(q_B,q_B')\in\ccalE$ are collected in a set $\ccalQ_F^{\text{dec}}$.%, i.e.,

Similar to \cite{bisoffi2018hybrid}, we define the distance of any state $q_B\in\ccalV$ to the set $\ccalV_F\subseteq \ccalV$ as
\begin{equation}\label{eq:distF}
d_F(q_B,\ccalV_F)=\min_{q_B'\in\ccalV_F}d(q_B,q_B'),
\end{equation}
where $d(q_B,q_B')$ is defined in \eqref{eq:dist} and $\ccalV_F$ is defined in \eqref{eq:accNode}; see also Fig.~\ref{fig:graphG}.

\subsection{Online Symbolic Controller}
\label{appendix:planning}

In this Section, we present how manipulation commands are generated online. The proposed controller requires as an input the graph $\ccalG$ defined in Appendix~\ref{sec:dist}. The main idea is that as the robot navigates the unknown environment, it selects NBA states that it should visit next so that the distance to the final states, as per \eqref{eq:distF}, decreases over time. 

Let $q_B(t)\in\ccalV$ be the NBA state that the robot has reached after navigating the unknown environment for $t$ time units. At time $t=0$, $q_B(t)$ is selected to be the initial NBA state. Given the current NBA state $q_B(t)$, the robot selects a new NBA state, denoted by $q_B^{\text{next}}\in\ccalV$ that it should reach next to make progress towards accomplishing their task. This state is selected among the neighbors of $q_B(t)$ in the graph $\ccalG$ based on the following two cases.
If $q_B(t)\notin \ccalV_F$, where $\ccalV_F$ is defined in \eqref{eq:accNode}, then among all neighboring nodes, we select one that satisfies
%$q_B^{\text{next}}\in\ccalQ_{q_B}^{\text{next}}\subseteq \ccalQ_B^{\text{dec}}$
\begin{equation}\label{eq:minDist}
d_F(q_B^{\text{next}},\ccalV_F) =  d_F(q_B(t),\ccalV_F)-1,  
\end{equation}
i.e., a state that is one hop closer to the set $\ccalV_F$ than $q_B(t)$ is where $d_F$ is defined in \eqref{eq:distF}.  Under this policy of selecting $q_B^{\text{next}}$, we have that eventually $q_B(t)\in\ccalV_F$; controlling the robot to ensure this property is discussed in Section~\ref{sec:reactive_planner}. If $q_B(t)\in\ccalV_F$, then the state $q_B^{\text{next}}$ is selected so that $(q_B(t),q_B^{\text{next}})$ is an accepting edge as per Definition~\ref{def:accEdges}. This way we ensure that accepting edges are traversed infinitely often and, therefore, the assigned LTL task is satisfied.

Given the selected state $q_B^{\text{next}}$, a feasible symbol is selected that can enable the transition from $q_B(t)$ to $q_B^{\text{next}}$, i.e., can incur the run \eqref{eq:run}. By definition of the run in \eqref{eq:run}, it suffices to select a symbol that satisfies the following Boolean formula:
\begin{equation}\label{eq:b}
   b^{q_B,q_B'}=b^{q_B,q_B^1}\wedge b^{q_B^2,q_B^3}\wedge\dots b^{q_B^{K-1},q_B^{K}}\wedge b^{q_B^{K},q_B^{K}},
\end{equation}
where $q_B^{K} = q_B^{\text{next}}$. In words, the Boolean formula in \eqref{eq:b} is the conjunction of all Boolean formulas $b^{q_B^{k-1},q_B^{k}}$ that need to be satisfied simultaneously to reach $q_B^{\text{next}}=q_B^K$ through a multi-hop path. Once such a symbol is generated, a point-to-point navigation and manipulation command is accordingly generated. For instance, if this symbol is $\pi^{a_k(\movableobjectdilated_i,\ell_j)}$ then the robot has to
apply the action $a_k(\movableobjectdilated_i,\ell_j)$, i.e.,
go to a known region of interest $\ell_j$ and apply action $a_k$ to the movable object $\movableobjectdilated_i$. The online implementation of such action is discussed in Section~\ref{sec:reactive_planner}. %By definition of \eqref{eq:b}, if there exists a feasible symbol $\sigma^{q_B,q_B'}$ that satisfies $b^{q_B,q_B'}$ then the finite word generated by repeating $K+1$ times the symbol $\sigma^{q_B,q_B'}$ can yield the run in \eqref{eq:run}.

%[+add a few words about completeness of this method+]
\subsection{Completeness of the Symbolic Controller}
\label{appendix:completeness}
In what follows, we provide the proof of Proposition~\ref{proposition:completeness}.

\begin{proof}[Proof of Proposition~\ref{proposition:completeness}]
To show this result it suffices to show that eventually the accepting condition of the NBA is satisfied, i.e., the robot will visit at least one of the final NBA states $q_F$ infinitely often. Equivalently, as discussed in Appendix~\ref{sec:dist}, it suffices to show that accepting edges $(q_B,q_B')\in\ccalE$, where $q_B,q_B'\in\ccalV$ are traversed infinitely often. 

First, consider an infinite sequence of time instants $\bbt=t_0,t_1,\dots,t_k,\dots$ where $t_{k+1}\geq t_k$, so that an edge in $\ccalG$, defined in Appendix~\ref{sec:dist}, is traversed at every time instant $t_k$. Let $e(t_k)\in\ccalE$ denote the edge that is traversed at time $t_k$. Thus, $\bbt$ yields the following sequence of edges $\bbe=e(t_0),e(t_1),\dots,e(t_k)\dots$ where $e(t_k)=(q_B(t_{k}),q_B(t_{k+1}))$, $q_B(t_0)=q_B^{\text{aux}}$, $q_B(t_k)\in\ccalV$, and the state $q_B^{k+1}$ is defined based on the following two cases. 
If $q_B(t_k)\notin \ccalV_F$, then the state $q_B(t_{k+1})$ is closer to $\ccalV_F$ than $q_B(t_k)$ is, i.e., $d_F(q_B(t_{k+1}),\ccalV_F)=d_F(q_B(t_{k}),\ccalV_F)-1$, where $d_F$ is defined in \eqref{eq:distF}. If $q_B(t_{k})\in\ccalV_F$, then $q_B(t_{k+1})$  is selected so that an accepting edge originating from $q_B(t_{k})$ is traversed. By definition of $q_B(t_{k})$, the `distance' to $\ccalV_F$ decreases as $t_k$ increases, i.e., given any time instant $t_k$, there exists a time instant $t_k'\geq t_k$ so that $q_B(t_{k}')\in\ccalV_F$ and then at the next time instant an accepting edge is traversed. This means that $\bbe$ includes an infinite number of accepting edges. This sequence $\bbe$ exists since, by assumption, there exists an infinite sequence of manipulation actions that satisfies $\phi$. Particularly, recall that by construction of the graph $\ccalG$, the set of edges in this graph captures all NBA transitions besides those that (i) require the robot to be in more than one region simultaneously or (ii) multi-hop NBA transitions that require the robot to jump instantaneously from one region of interest which are not meaningful in practice. As a result, if there does not exist at least one sequence $\bbe$, i.e., at least one infinite path in $\ccalG$ that starts from the initial state and traverses at least one accepting edge infinitely often, then this means that there is no path that satisfies $\phi$ (unless conditions (i)-(ii) mentioned before are violated).  %Note that if assumption (a) does not hold, the proposed discrete controller cannot find a solution.

%that there exists a solution to the considered problem, i.e., an infinite sequence of manipulation commands generated by the discrete controller that satisfy the assigned LTL formula $\phi$. 
Assume that the discrete controller selects NBA states as discussed in Appendix~\ref{appendix:planning}. To show that the discrete controller is complete, it suffices to show that it can generate a infinite sequence of edges $\bbe$ as defined before. Note that the discrete controller selects next NBA states that the robot should reach in the same way as discussed before. Also, by assumption, the environmental structure and the continuous-time controller ensure that at least one of the candidate next NBA states (i.e., the ones that can decrease the distance to $\ccalV_F$) can be reached. Based on these two observations, we conclude that such a sequence $\bbe$ will be generated, %as long as the continuous-time controller and the environmental structure allow the robot to accomplish the manipulation commands required to enable the transitions from $q_B(t_{k})\in\ccalV$ to $q_B(t_{k+1})\in\ccalV$, for all $t_k$. However, this is guaranteed due to Assumption (b) 
completing the proof.
\end{proof}

%\textit{Assumption (a):} In words, Assumption (a) implies that there exists an infinite sequence of manipulation-based atomic predicates that if satisfied, then the accepting edges of $\ccalG$ will be traversed infinitely often (or equivalently, the set of accepting NBA states will be visited infinitely often), and, therefore, the LTL task will be satisfied. Recall that by construction of the graph $\ccalG$, the set of edges in this graph captures all NBA transitions besides those that (i) require the robot to  be in more than one region simultaneously or (ii) multi-hop NBA transitions that require the robot to jump instantaneously from one region of interest which are not meaningful in practice. As a result, if Assumption (a) does not hold, then this means that there is no path that satisfies $\phi$ (unless conditions (i)-(ii) mentioned before are violated). 

Note that the graph $\ccalG$ is agnostic to the structure of the environment, meaning that an edge in $\ccalG$ may not be able to be traversed. For instance, consider an edge in this graph that is enabled only if the robot applies a certain action to a movable object that is in a region blocked by fixed obstacles; in this case the continuous-time controller will not be able to execute this action due to the environmental structure. Satisfaction of the second assumption in Proposition~\ref{proposition:completeness} implies that if such scenarios never happen, (e.g., all regions and objects that the robot needs to interact with are accessible and the continuous-time controller allows the robot to reach them) then the proposed hybrid control method will satisfy the assigned LTL task if this formula is feasible. However, if the second assumption does not hold,  there may  be an alternative sequence of automaton states to follow in order to satisfy the LTL formula that the proposed algorithm failed to find due to the \`a-priori unknown structure of the environment.
