# Supplementary material for: Reactive Informative Planning for Mobile Manipulation Tasks under Sensing and Environmental Uncertainty
Source: arXiv:2205.06301 source file (2022-05-12)
Supplement: Supplementary file 2 [file appendix_reactive_planner.tex]

\section{Reactive Controller Overview}
\label{appendix:reactive_controller_overview}

This Appendix provides a brief description of the reactive, vector field controller from \cite{vasilopoulos_pavlakos_bowman_caporale_daniilidis_pappas_koditschek_2020} used in this work. As shown in Fig.~\ref{fig:simulation_simple}, the robot navigates the physical space and discovers obstacles (e.g., using the semantic mapping engine in \cite{Bowman2017}), which are dilated by the robot radius and stored in the semantic space. Potentially overlapping obstacles in the semantic space are subsequently consolidated in real time to form the mapped space. A change of coordinates $\diffeogeneric$ from this space is then employed to construct a geometrically simplified (but topologically equivalent) model space, by merging familiar obstacles overlapping with the boundary of the enclosing freespace to this boundary, deforming other familiar obstacles to disks, and leaving unknown obstacles intact. It is shown in \cite{vasilopoulos_pavlakos_bowman_caporale_daniilidis_pappas_koditschek_2020} that the constructed change of coordinates $\diffeo$ between the mapped and the model space, for a given index set $\hybridmode$ of instantiated familiar obstacles, is a $C^\infty$ diffeomorphism away from sharp corners. Using the diffeomorphism $\diffeo$, we construct a hybrid vector field controller (with the modes indexed by $\hybridmode$, i.e., depending on external perceptual updates), that guarantees simultaneous obstacle avoidance and target convergence, while respecting input command limits, in unexplored semantic environments (see \cite[Eq. (1)]{vasilopoulos_pavlakos_bowman_caporale_daniilidis_pappas_koditschek_2020}). The reactive controller is further extended to accommodate differential-drive robot dynamics, while maintaining the same formal guarantees.

\section{Description of the Topology Checking Algorithm}
\label{appendix:topology_checking_algorithm}

This Appendix includes an algorithmic outline of the topology checking algorithm from Section~\ref{subsec:topology_checking}, shown in Algorithm~\ref{algorithm:topology_checking}. This algorithm works as follows. Starting with the initially assumed polygonal enclosing freespace $\enclosingfreespace$ for either the robot or the robot-object pair, we subtract the union of all known dilated movable objects in $\movableobjectsetdilated$ and fixed obstacles in $\knownobstaclesetdilated_\hybridmode$ (corresponding to the index set $\hybridmode$ of localized familiar obstacles), using standard logic operations with polygons (see e.g., \cite{elgindy_1993,clementini_1993,douglas_1973}). This operation results in a list of freespace components, which we denote by $\mathcal{L}_\freespace := (\freespace_1, \freespace_2, \ldots)$. From this list, we identify the freespace $\freespace$ as the freespace component $\freespace_k$ that contains the robot position $\robotposition$ (or the robot-object pair center $\robotposition_{i,c}$) and re-define the enclosing freespace as its convex hull, i.e., $\enclosingfreespace := \text{Conv}\left(\overline{\freespace}_k\right)$.

If the goal $\goalposition$ is contained in $\enclosingfreespace$, the reactive controller proceeds as usual, using $\enclosingfreespace$ for the diffeomorphism construction (see Appendix~\ref{appendix:reactive_controller_overview}), and treating all other freespace components as obstacles. Otherwise, we need to check whether movable objects or fixed obstacles cause a freespace disconnection that does not allow for successful action completion. Namely, we need to check whether both the robot position $\robotposition$ (or the robot-object pair center $\robotposition_{i,c}$) and the target $\goalposition$ are included in the same connected component of the set $\mathcal{L}_{\freespace+\movableobjectsetdilated} := \left(\bigcup_i \freespace_i\right) \cup \left(\bigcup_j \movableobjectdilated_j\right)$, i.e., the union of all freespace components in $\mathcal{L}_\freespace$ with all dilated movable objects in $\movableobjectsetdilated$. This would imply that a subset of movable objects in $\movableobjectsetdilated$ blocks the target configuration. In that case, the robot switches to the Fix mode to rearrange these objects; otherwise, the interface layer reports to the symbolic controller that the current action is infeasible.

In the former case, we proceed one step further to identify the blocking movable objects in order to reconfigure them on-the-fly. First, we isolate the connected components of the union of all movable objects in $\movableobjectsetdilated$ into a list $\mathcal{L}_{\movableobjectsetdilated} := (\movableobjectsetdilated_1, \movableobjectsetdilated_2, \ldots)$; we refer to the elements of that list as the {\it movable object clusters}. Assuming that each movable object cluster is connected to at most two freespace components from $\mathcal{L}_\freespace$, we build a connectivity tree rooted at the robot's (or the robot-object pair's) freespace $\freespace$, by checking whether the closures of two individual regions overlap; the tree's vertices are geometric regions (freespace components in $\mathcal{L}_\freespace$ and movable object clusters in $\mathcal{L}_{\movableobjectsetdilated}$) and edges denote adjacency. We then backtrack from the vertex of the tree that contains the goal $\goalposition$ until we reach the root, saving the encountered movable object clusters along the way. Any movable object intersecting any of these clusters is pushed to a stack of {\it blocking movable objects} $\mathcal{B}_{\movableobjectsetdilated}$.

\begin{algorithm}
\begin{algorithmic}
\Function{TopologyChecking}{$\robotposition$,$\goalposition$,$\enclosingfreespace$,$\movableobjectsetdilated$,$\knownobstaclesetdilated_\hybridmode$}
\State $\mathcal{L}_\freespace \gets \texttt{Subtract}(\enclosingfreespace,\texttt{Union}(\movableobjectsetdilated,\knownobstaclesetdilated_\hybridmode$))
\For{$\freespace_k \in \mathcal{L}_\freespace$}
\If{$\robotposition \in \freespace_k$}
\State $\freespace \gets \freespace_k$
\State $\enclosingfreespace \gets \text{Conv}(\overline{\freespace}_k)$
\State $\textbf{break}$
\EndIf
\EndFor
\If{$\goalposition \in \freespace$}
\State $\mathcal{B}_\movableobjectsetdilated \gets \varnothing$ \Comment{No blocking objects or obstacles}
\State $\texttt{IsFeasible} \gets \texttt{True}$ \Comment{Task feasible}
\Else
\State $\mathcal{L}_{\freespace+\movableobjectsetdilated} \gets (\bigcup_i \freespace_i) \cup (\bigcup_j \movableobjectdilated_j), \mathcal{F}_i \in \mathcal{L}_\freespace, \movableobjectdilated_j \in \movableobjectsetdilated$
\For{$\freespace_k \in \mathcal{L}_{\freespace+\movableobjectsetdilated}$}
\If{$\robotposition \in \freespace_k$}
\If{$\goalposition \in \freespace_k$}
\State $\mathcal{L}_\movableobjectsetdilated \gets \bigcup_j \movableobjectdilated_j, \movableobjectdilated_j \in \movableobjectsetdilated$
\State $(\mathcal{V}_\mathcal{L},\mathcal{E}_\mathcal{L}) \gets \texttt{ConnectTree}(\mathcal{L}_\freespace,\mathcal{L}_\movableobjectsetdilated)$
\For{$V \in \mathcal{V}_\mathcal{L}$}
\If{$\goalposition \in V$}
\State $\mathcal{B}_\movableobjectsetdilated \gets \texttt{BacktrackFrom}(V)$
\State $\textbf{break}$
\EndIf
\EndFor
\State $\texttt{IsFeasible} \gets \texttt{True}$
\Else
\State $\mathcal{B}_\movableobjectsetdilated \gets \varnothing$ \Comment{Blocked by fixed obstacles}
\State $\texttt{IsFeasible} \gets \texttt{False}$
\EndIf
\State $\textbf{break}$
\EndIf
\EndFor
\EndIf
\State $\textbf{return} \quad \enclosingfreespace, \texttt{IsFeasible}, \mathcal{B}_\movableobjectsetdilated$
\EndFunction
\end{algorithmic}
\caption{Topology Checking Algorithm.} \label{algorithm:topology_checking}
\end{algorithm}
